# Supplementary material for: On the Energy Consumption of Test Generation
Source: arXiv:2501.09657 source file (2025-01-16)
Supplement: Supplementary file 1 [file appendix.tex]

\todo[inline]{These tables are too large/too many to be included. For Tab.~\ref{tab:energy_boxplot} we could add only significant pairs. For tables about dominance we could hae relevant values in the text.}

Tab.~\ref{tab:energy_boxplot} performs Wilcoxon test on the data presented in Fig.~\ref{fig:energy_boxplot}. Columns are:
\begin{itemize}
    \item g1 and g2 are the two boxplots in Fig.~\ref{fig:energy_boxplot} compared;
    \item pval, VD.A and Mag are the p-value of Wilcoxon test, the Vargha-Delaney statistics, and the magnitude of Vargha-Delaney, respectively;
    \item en\_g1 and en\_g2 are the median energy of groups g1 and g2, respectively;
    \item aggregate represents the value used to aggregate data for comparison. In the first row, Low CCN  and High CCN are compared for algorithm RANDOM\_SEARCH;
    \item cov says if the row refers to the cases with coverage less 100\% or not, so left or right group of boxplots;
    \item p\_adjust is the adjusted pvalue with FDR method.
\end{itemize}

For instance, the first row says that for RANDOM\_SEARCH in cases with Cov $<$ 100, there is no significant difference in energy consumption when generating tests for Low CCN  or High CCN, as p\_adjust is 0.161. Instead, when considering  MU\_PLUS\_LAMBDA\_EA, the difference in energy consumption is significant (p\_adjust 0.000 means < 0.001). A different comparison is from line 11, where energy consumption of RANDOM\_SEARCH and DYNAMOSA are compared for Low CCN classes and Cov $<$ 100\% returning an adjusted p-value greater than 0.008.

Pairwise comparison data: a table for each algorithm in which the algorithm is compared with the others. Total dominance: better coverage and better energy. Energy dominance: same coverage but better energy. We'll show a table for each algorithm that presents the comparison data with all the other algorithms: \mosa Tab.~\ref{tab:pairwise_dynamosa}, \mupluslambda Tab.~\ref{tab:pairwise_mulambda}, \nsga Tab.~\ref{tab:pairwise_nsgaii}, \rnd Tab.~\ref{tab:pairwise_rnd}, and \steady Tab.~\ref{tab:pairwise_steady}.

\begin{table*}[htb]
\centering
\begingroup\fontsize{6pt}{7pt}\selectfont
\begin{tabular}{lrrr}
  \hline
alg & total\_dominance & energy\_dominance & n\_classes \\ 
  \hline
Mu+Lambda & 6 & 73 & 348 \\ 
  NSGAII & 32 & 260 & 348 \\ 
  Random & 15 & 30 & 348 \\ 
  Steady-State & 23 & 235 & 348 \\ 
   \hline
\end{tabular}
\endgroup
\caption{Dynamosa}
\label{tab:pairwise_dynamosa}
\end{table*}

\begin{table*}[htb]
\centering
\begingroup\fontsize{6pt}{7pt}\selectfont
\begin{tabular}{lrrr}
  \hline
alg & total\_dominance & energy\_dominance & n\_classes \\ 
  \hline
Dynamosa & 3 & 177 & 348 \\ 
  NSGAII & 18 & 237 & 348 \\ 
  Random & 15 & 39 & 348 \\ 
  Steady-State & 16 & 224 & 348 \\ 
   \hline
\end{tabular}
\endgroup
\caption{Mu+Lambda}
\label{tab:pairwise_mulambda}
\end{table*}

\begin{table*}[htb]
\centering
\begingroup\fontsize{6pt}{7pt}\selectfont
\begin{tabular}{lrrr}
  \hline
alg & total\_dominance & energy\_dominance & n\_classes \\ 
  \hline
Dynamosa & 1 & 11 & 348 \\ 
  Mu+Lambda & 2 & 48 & 348 \\ 
  Random & 4 & 8 & 348 \\ 
  Steady-State & 2 & 18 & 348 \\
   \hline
\end{tabular}
\endgroup
\caption{NSGAII}
\label{tab:pairwise_nsgaii}
\end{table*}

\begin{table*}[htb]
\centering
\begingroup\fontsize{6pt}{7pt}\selectfont
\begin{tabular}{lrrr}
  \hline
alg & total\_dominance & energy\_dominance & n\_classes \\ 
  \hline
Dynamosa & 3 & 231 & 348 \\ 
  Mu+Lambda & 0 & 169 & 348 \\ 
  NSGAII & 15 & 263 & 348 \\ 
  Steady-State & 6 & 256 & 348 \\ 
   \hline
\end{tabular}
\endgroup
\caption{Random}
\label{tab:pairwise_rnd}
\end{table*}

\begin{table*}[htb]
\centering
\begingroup\fontsize{6pt}{7pt}\selectfont
\begin{tabular}{lrrr}
  \hline
alg & total\_dominance & energy\_dominance & n\_classes \\ 
  \hline
Dynamosa & 1 & 25 & 348 \\ 
  Mu+Lambda & 1 & 51 & 348 \\ 
  NSGAII & 13 & 206 & 348 \\ 
  Random & 5 & 23 & 348 \\ 
   \hline
\end{tabular}
\endgroup
\caption{Steady-State}
\label{tab:pairwise_steady}
\end{table*}

\clearpage

\begin{table*}[htb]
\centering
\begingroup\fontsize{6pt}{6pt}\selectfont
\begin{tabular}{lrrrrrrr}
  \hline
project\_name & median\_manual & median\_auto & pval & avg\_ccn\_manual & avg\_ccn\_auto & max\_ccn\_manual & max\_ccn\_auto \\ 
  \hline
imglib-imglib2 & 201.118 & 1862.861 & 0.000 & 1.864 & 1.450 &   17 &    8 \\ 
  Wolfgang-Schuetzelhofer-jcypher & 5012.817 & 588.582 & 0.000 & 2.311 & 1.164 &   29 &    3 \\ 
  geophile-geophile & 17481.481 & 49.229 & 0.000 & 1.975 & 1.244 &   18 &    2 \\ 
  albertoirurueta-irurueta-geometry & 23001.006 & 36.799 & 0.000 & 3.603 & 1.116 &   46 &    2 \\ 
  spullara-java-future-jdk8 & 6315.078 & 18.882 & 0.000 & 1.868 & 1.253 &   11 &    2 \\ 
  josueeduardo-rest-client & 11050.282 & 17.198 & 0.000 & 1.362 & 1.272 &    5 &    2 \\ 
  albertoirurueta-irurueta-navigation-indoor & 14599.956 & 15.429 & 0.000 & 4.765 & 1.161 &  135 &    2 \\ 
   \hline
\end{tabular}
\endgroup
\end{table*}
